# Supplementary material for: Inverse design of focused vector beams for mode excitation in optical nanoantennas
Source: arXiv:2204.07379 source file (2022-04-15)
Supplement: Supplementary file 1 [file SM.pdf]

# Inverse design of focused vector beams for mode excitation in optical nanoantennas–Supplemental Material

Xiaorun Zang,* Ari T. Friberg, Tero Setälä, and Jari Turunen
*Institute of Photonics, University of Eastern Finland, P.O. Box 111, FI-80101 Joensuu, Finland*
(Dated: March 20, 2022)

In the inverse design, the eigenmode's near field in the focal plane Γ is taken as the desired focal field. For choosing the appropriate components in the desired focal field that will unambiguously determine the beam-like pupil field and thus the designed focal field, we categorize the desired focal fields (as listed in the following table) according to the time-averaged energies associated with the transverse and longitudinal electric and magnetic fields in the focal plane, i.e., the surface integrals of the energy densities given in Eqs. (30)–(33).

| $\max(\mathscr{W}^{(m)}_{e,\text{tran}}, \mathscr{W}^{(m)}_{e,\text{long}}, \mathscr{W}^{(m)}_{h,\text{tran}}, \mathscr{W}^{(m)}_{h,\text{long}})$ | a nanodisk monomer | a nanodisk dimer | a nanodisk tetramer |
|---|---|---|---|
| $= \mathscr{W}^{(m)}_{e,\text{tran}}$, in group Ⓘ | M3–9 | M1–6,11,12 | M2–9,12 |
| $= \mathscr{W}^{(m)}_{e,\text{long}}$, in group (II) | M10 | - | - |
| $= \mathscr{W}^{(m)}_{h,\text{tran}}$, in group (III) | M1,2,11,12 | M7–10 | M10,11 |
| $= \mathscr{W}^{(m)}_{h,\text{long}}$, in group (IV) | - | - | M1 |

For the first twelve dominant eigenmodes in a nanodisk monomer, Figs. S1–S12 show all the electric and magnetic field components of a desired focal field in the real space (first column) and spatial frequency **k** space (second column), the designed pupil field (third column), and the designed focal field (fourth column). The desired focal field is evaluated in the focal plane, which is actually the eigenmode's near field calculated via Eqs. (19) and (20) in the maintext. For the first twelve leading eigenmodes in a nanodisk dimer and tetramer, electric and magnetic field components at different states of the inverse design are shown in a similar fashion in Figs. S13–S24 and Figs. S25–36, respectively.

* xiaorun.zang@aalto.fi; Currently at Department of Applied Physics, Aalto University, P.O Box 13500, FI-00076 Aalto, Finland

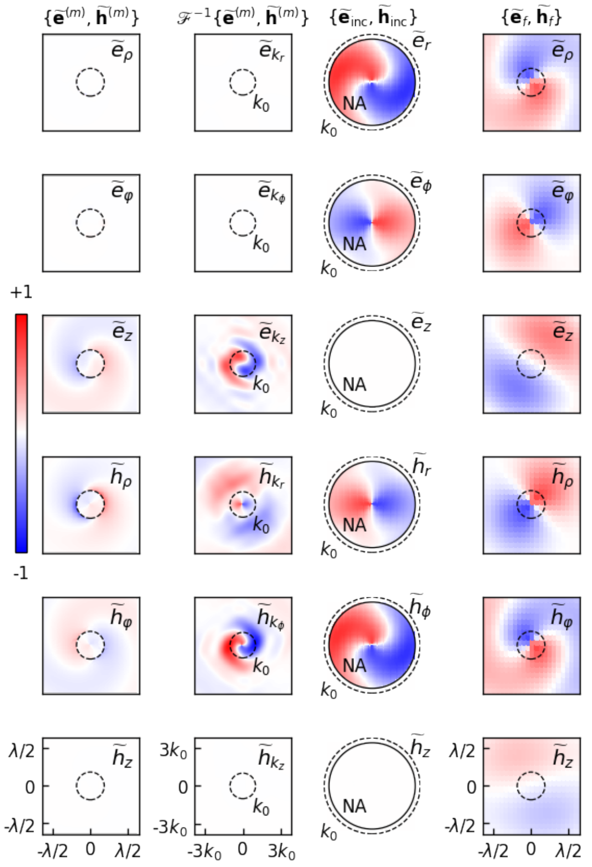


Figure S1. Fields for mode M1 in a nanodisk monomer.

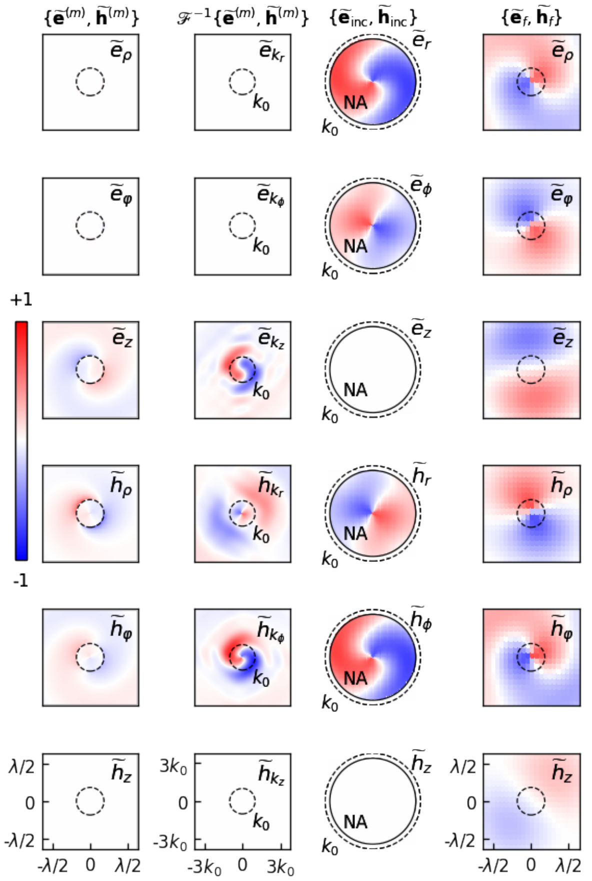


Figure S2. Fields for mode M2 in a nanodisk monomer.

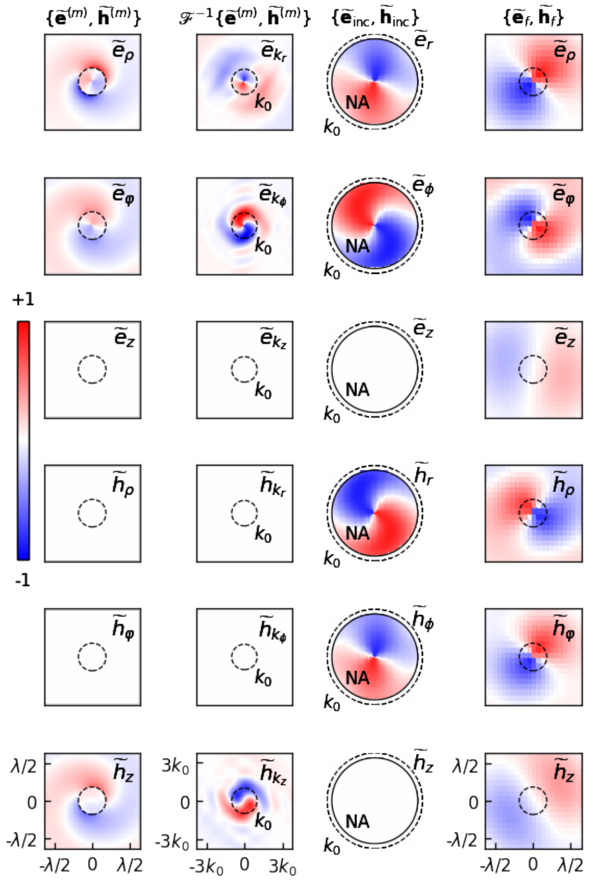


Figure S3. Fields for mode M3 in a nanodisk monomer.

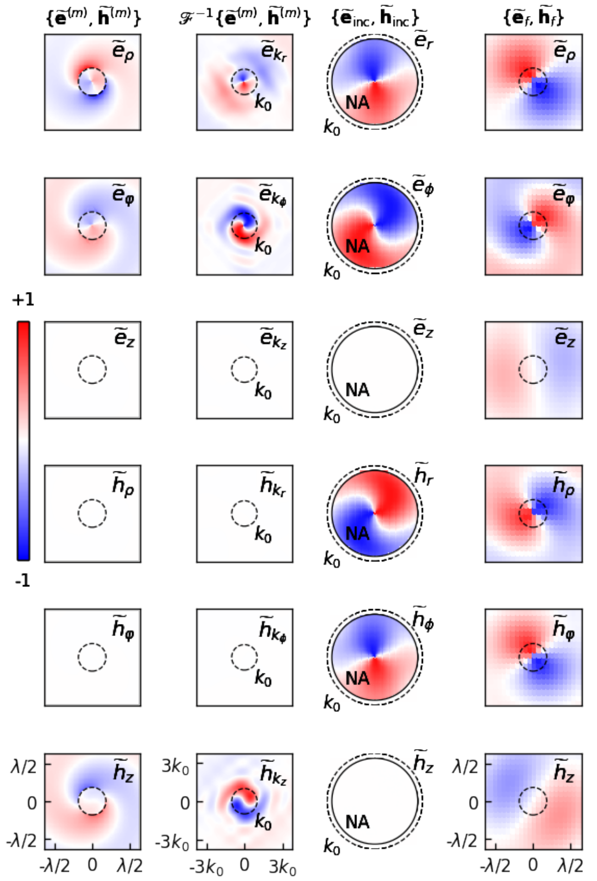


Figure S4. Fields for mode M4 in a nanodisk monomer.

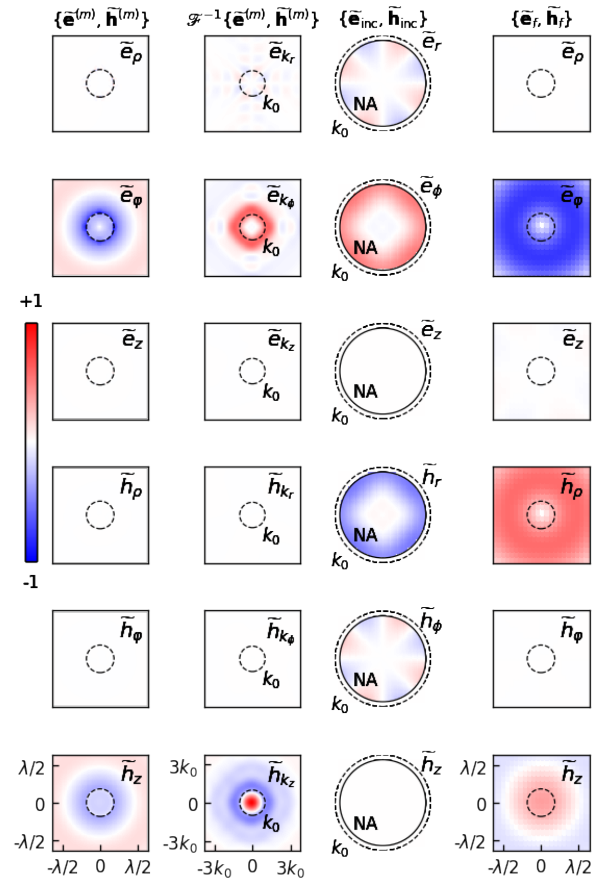


Figure S5. Fields for mode M5 in a nanodisk monomer.

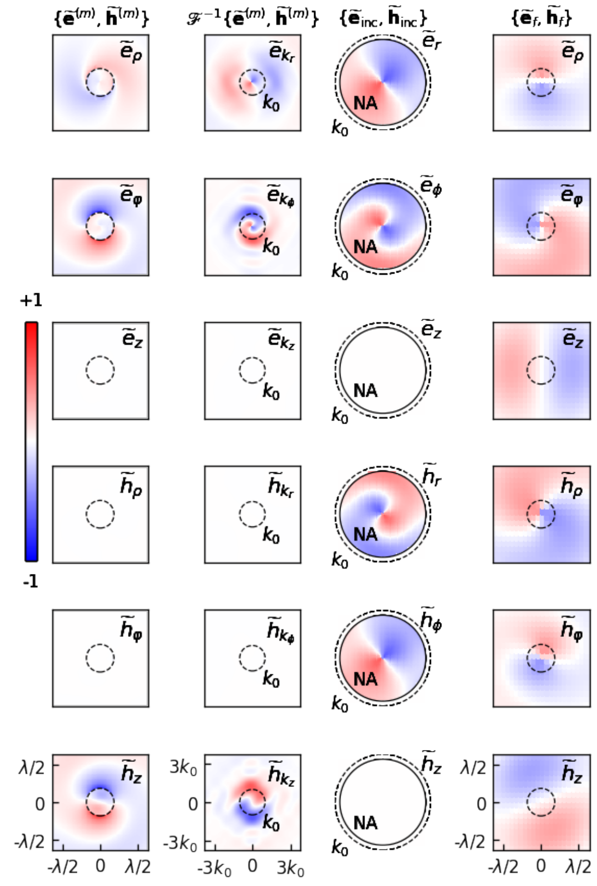


Figure S6. Fields for mode M6 in a nanodisk monomer.

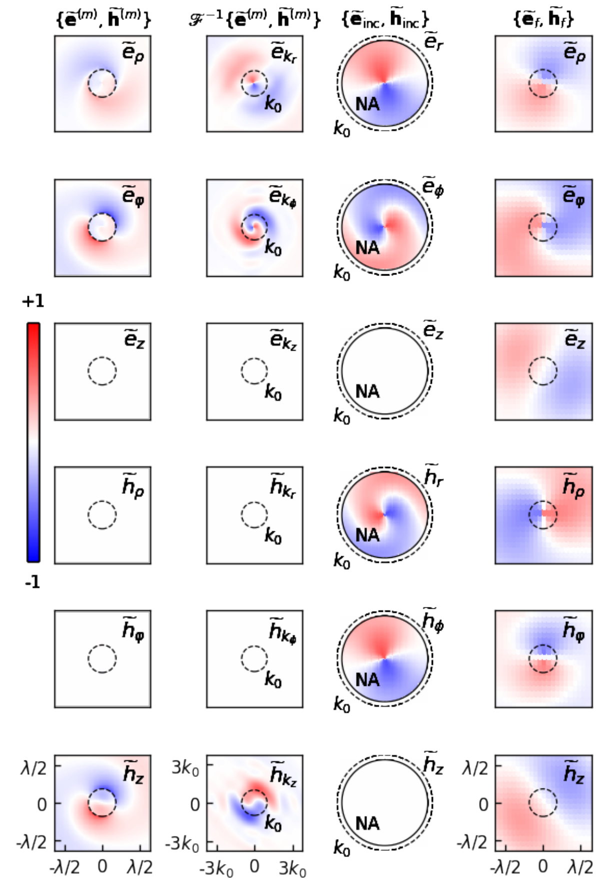


Figure S7. Fields for mode M7 in a nanodisk monomer.

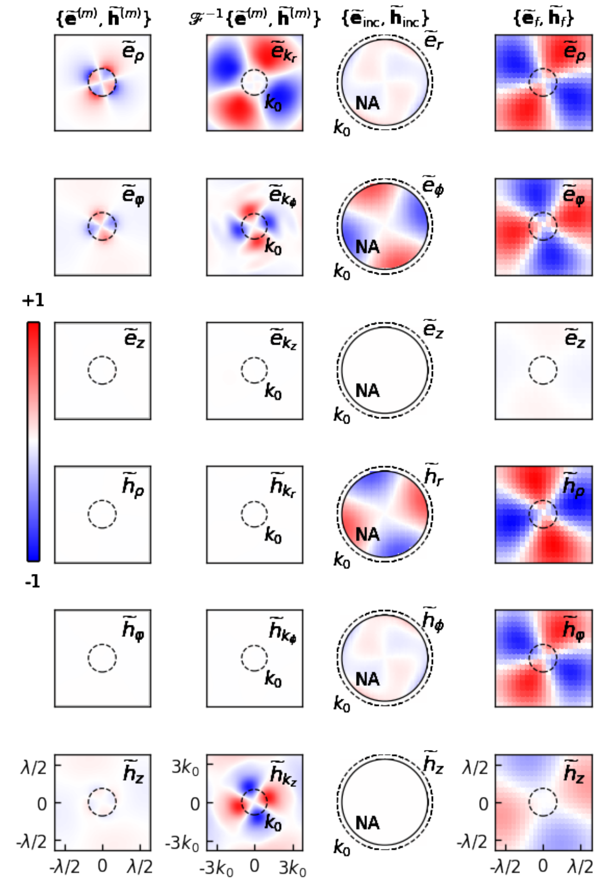


Figure S8. Fields for mode M8 in a nanodisk monomer.

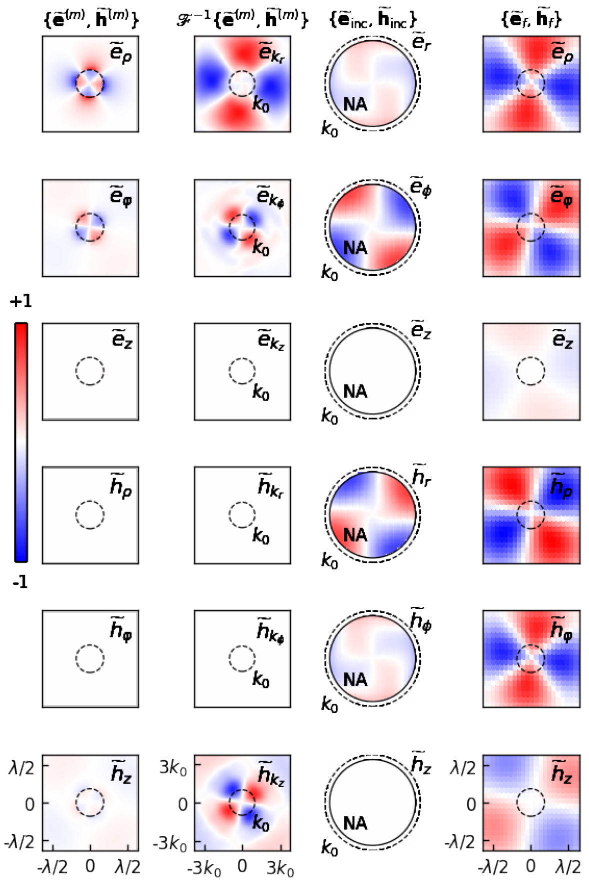


Figure S9. Fields for mode M9 in a nanodisk monomer.

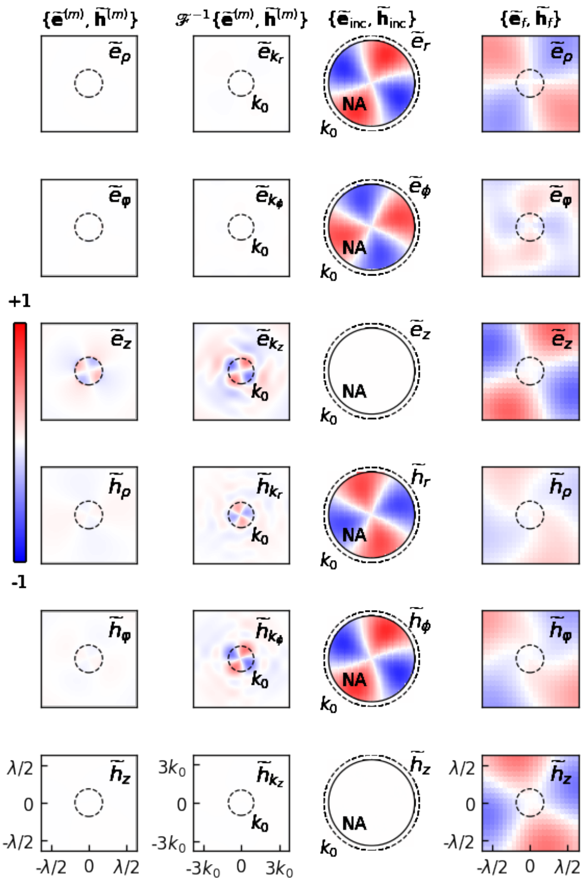


Figure S11. Fields for mode M11 in a nanodisk monomer.

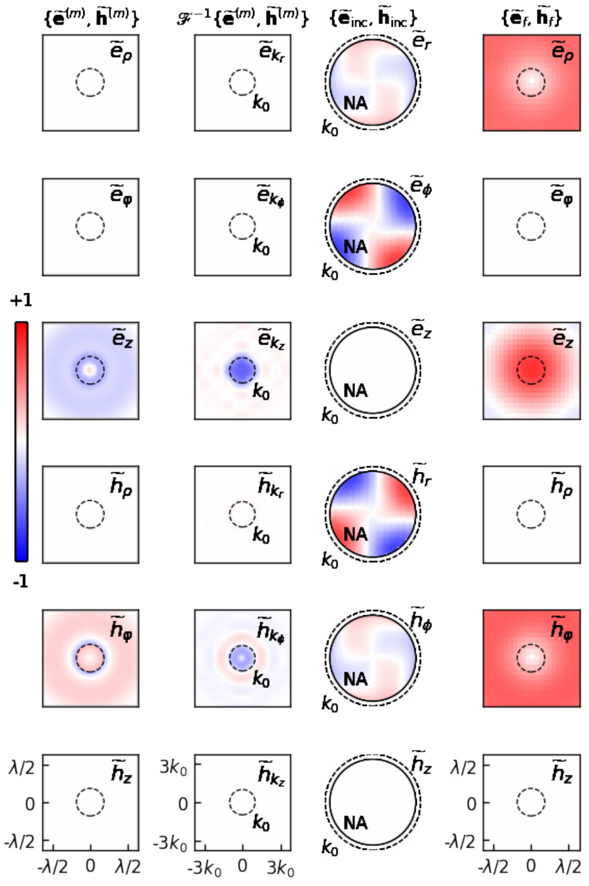


Figure S10. Fields for mode M10 in a nanodisk monomer.

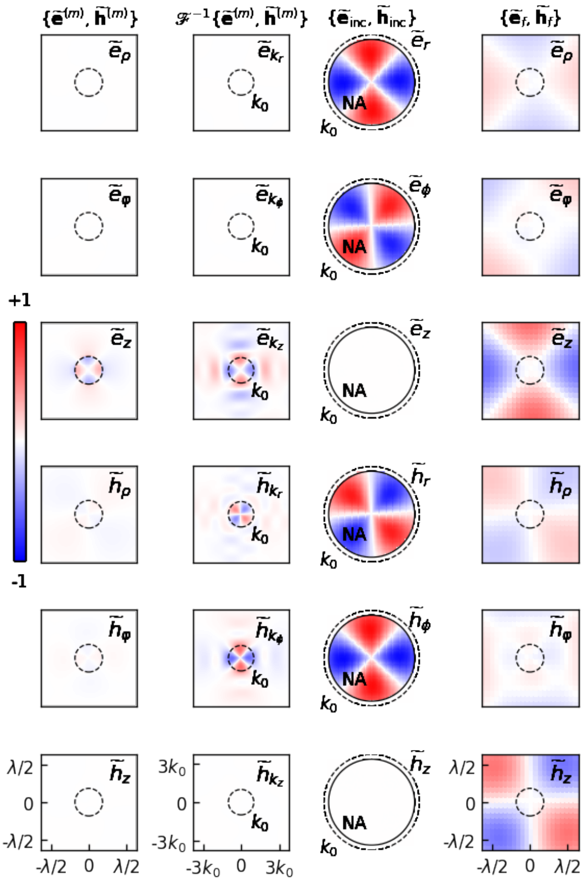


Figure S12. Fields for mode M12 in a nanodisk monomer.

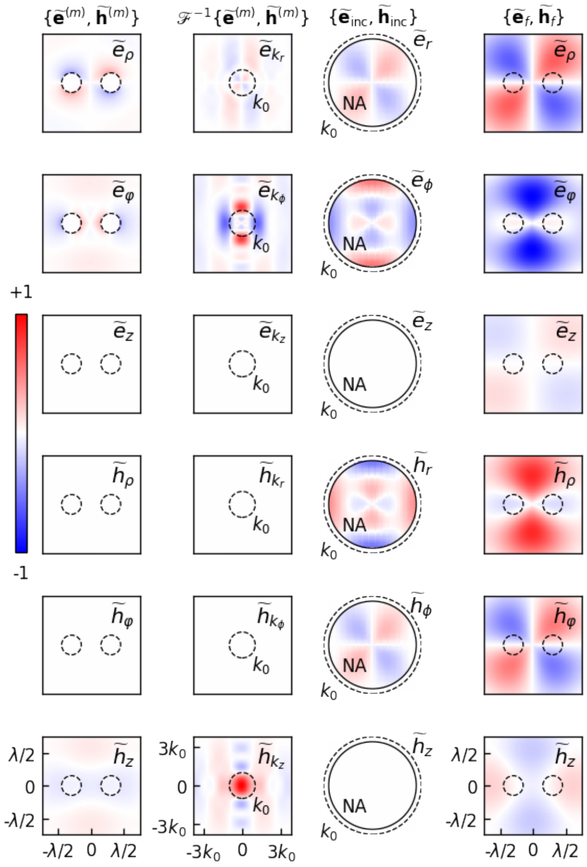


Figure S13. Fields for mode M1 in a nanodisk dimer.

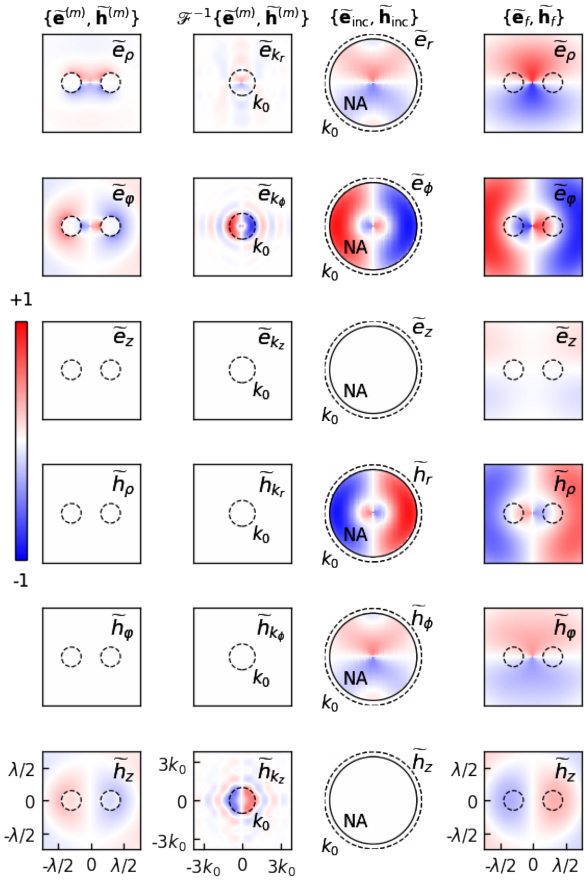


Figure S14. Fields for mode M2 in a nanodisk dimer.

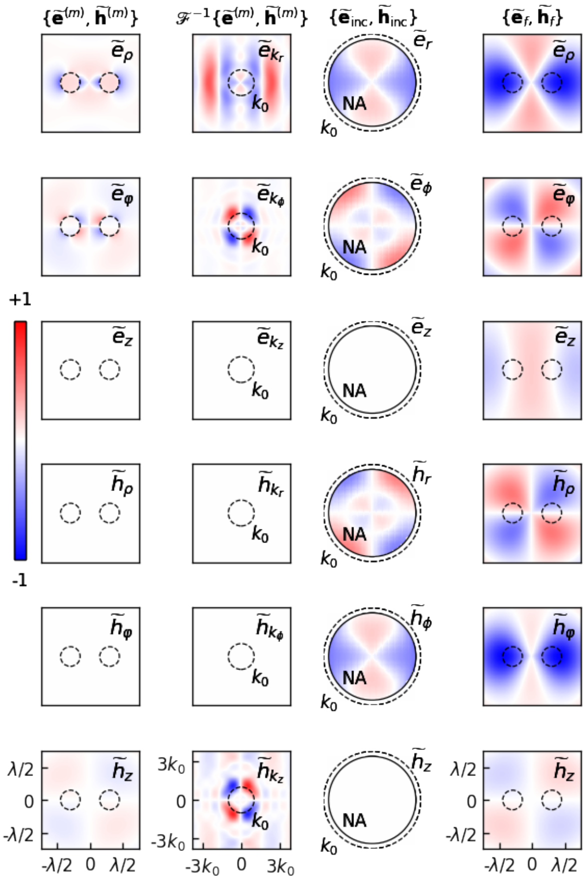


Figure S15. Fields for mode M3 in a nanodisk dimer.

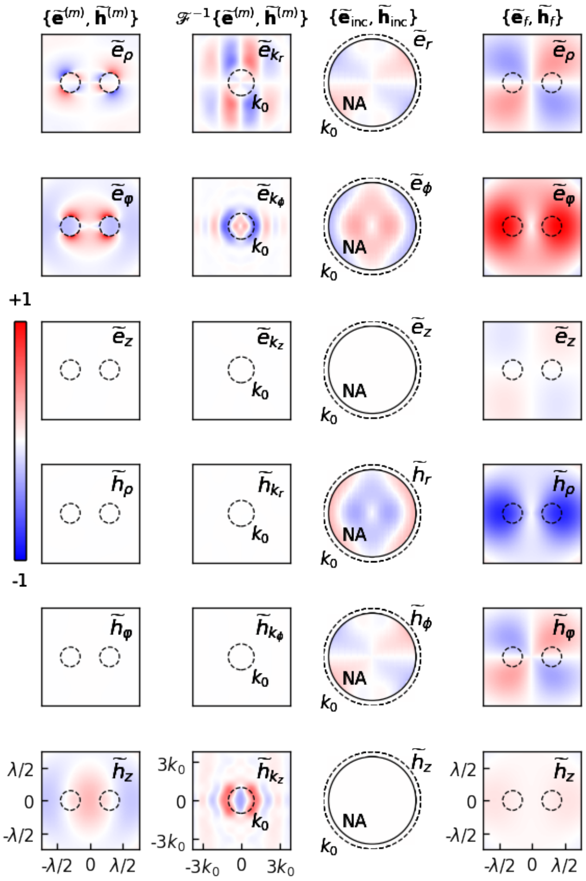


Figure S16. Fields for mode M4 in a nanodisk dimer.

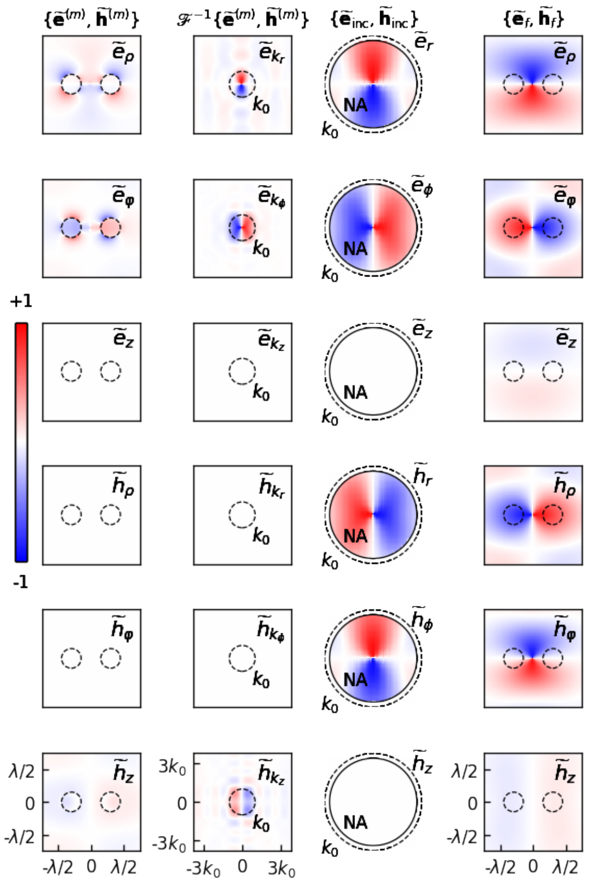


Figure S17. Fields for mode M5 in a nanodisk dimer.

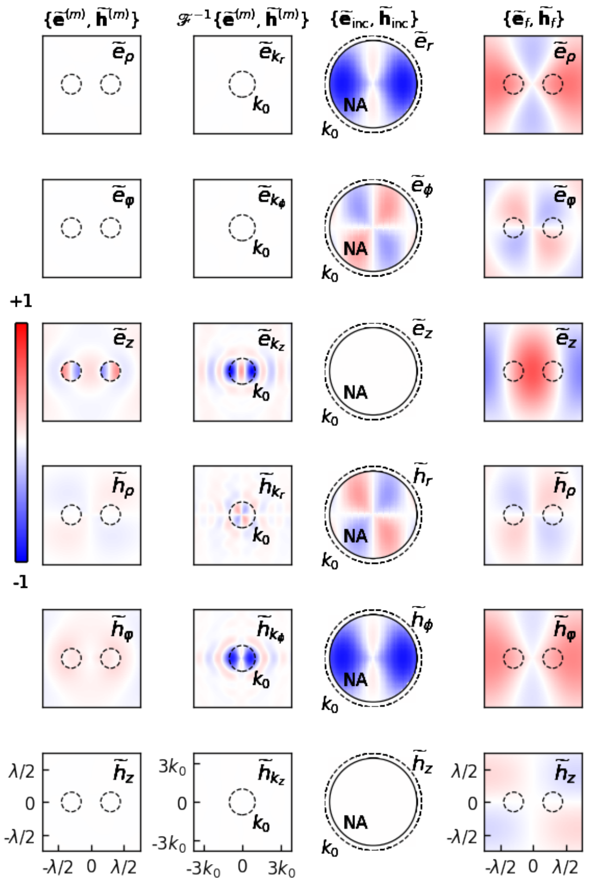


Figure S19. Fields for mode M7 in a nanodisk dimer.

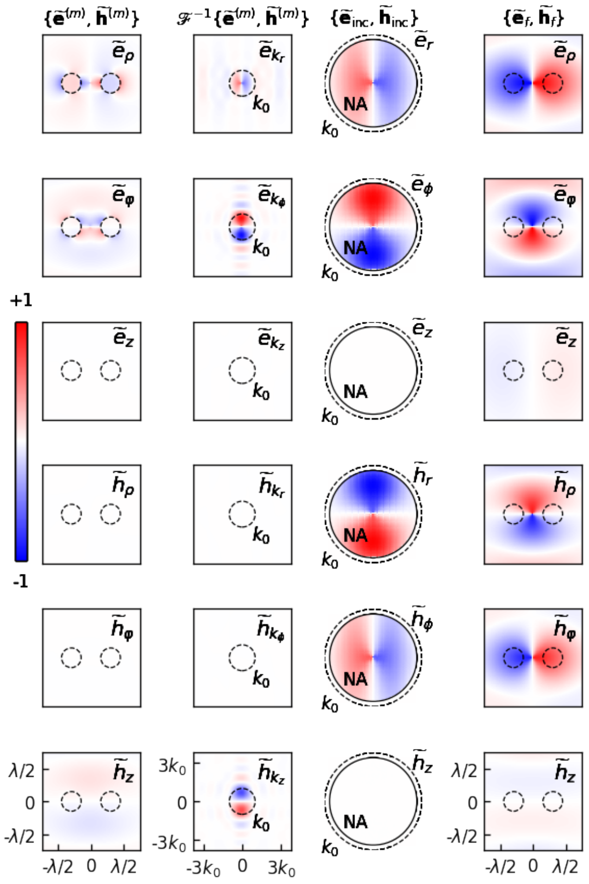


Figure S18. Fields for mode M6 in a nanodisk dimer.

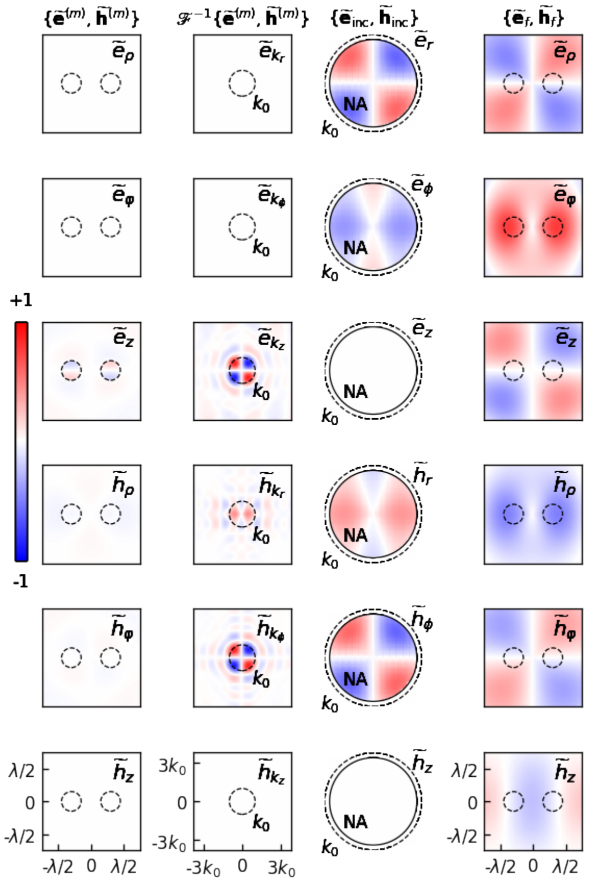


Figure S20. Fields for mode M8 in a nanodisk dimer.

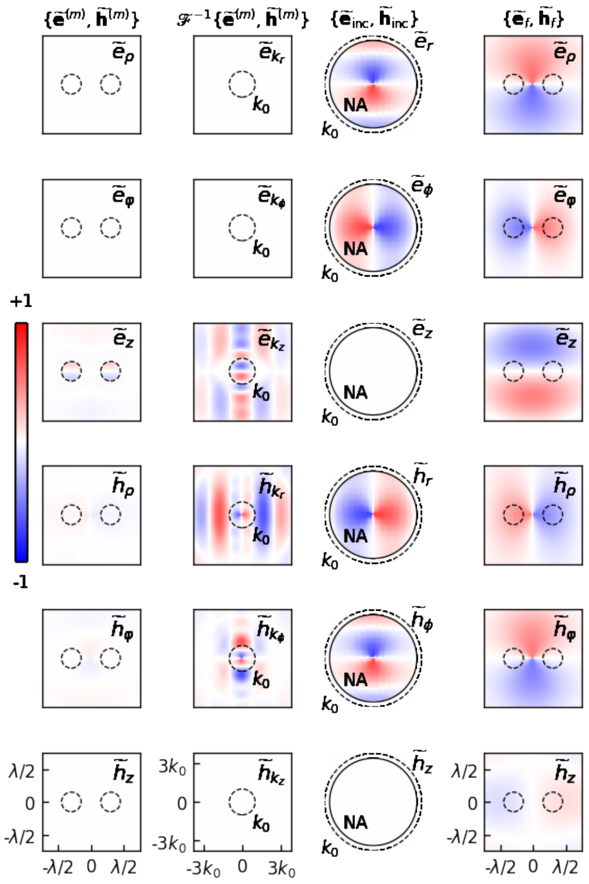


Figure S21. Fields for mode M9 in a nanodisk dimer.

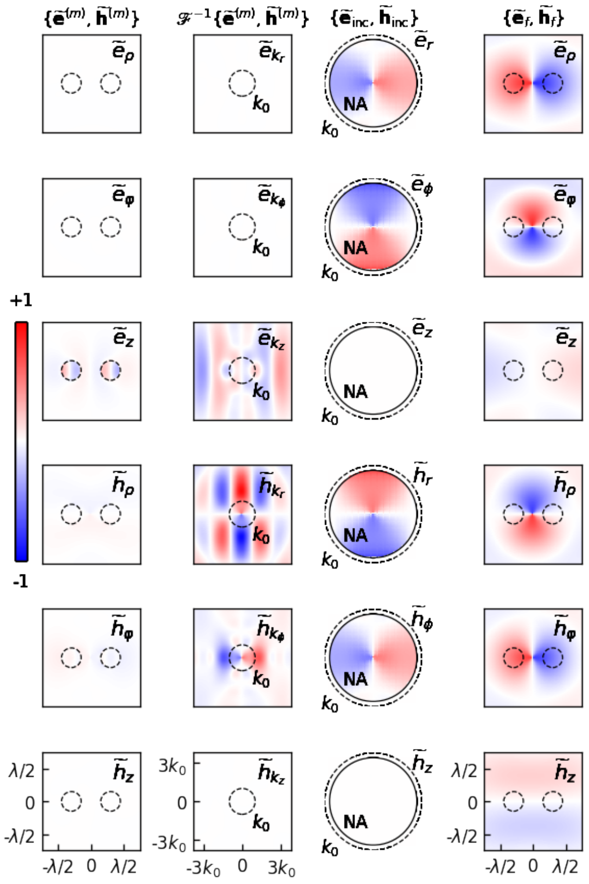


Figure S22. Fields for mode M10 in a nanodisk dimer.

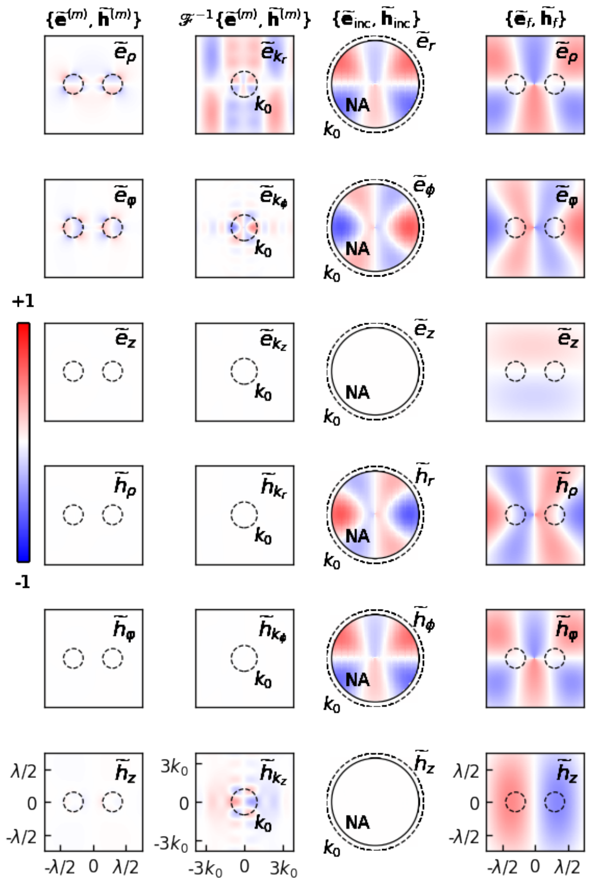


Figure S23. Fields for mode M11 in a nanodisk dimer.

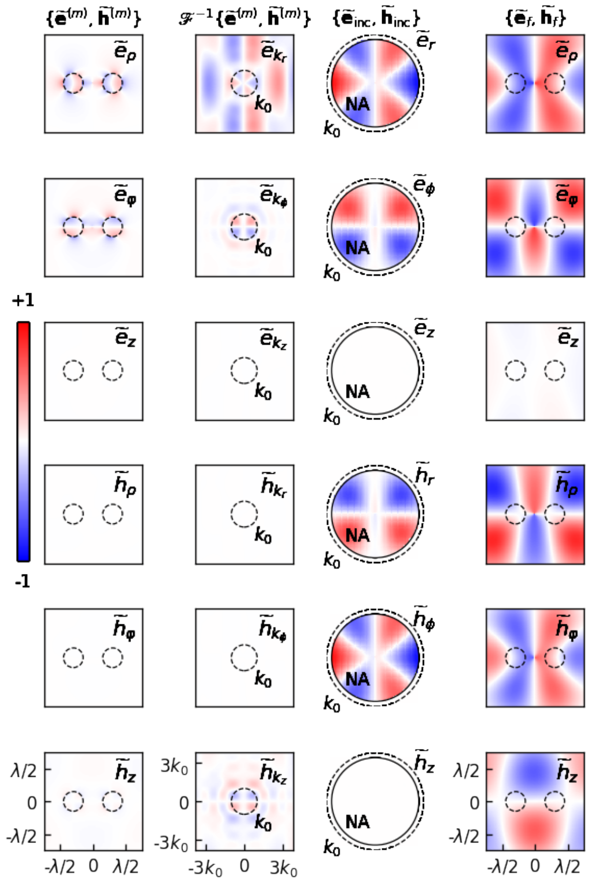


Figure S24. Fields for mode M12 in a nanodisk dimer.

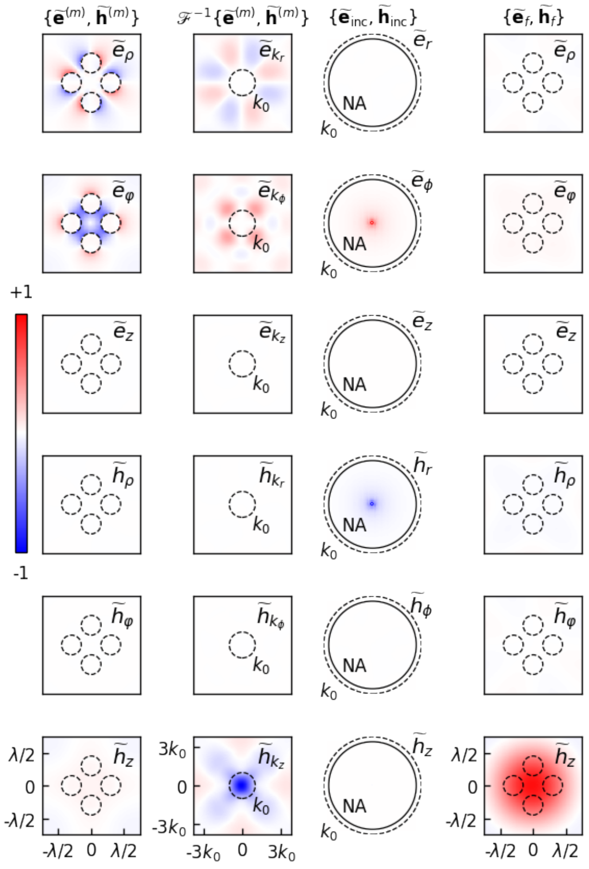


Figure S25. Fields for mode M1 in a nanodisk tetramer.

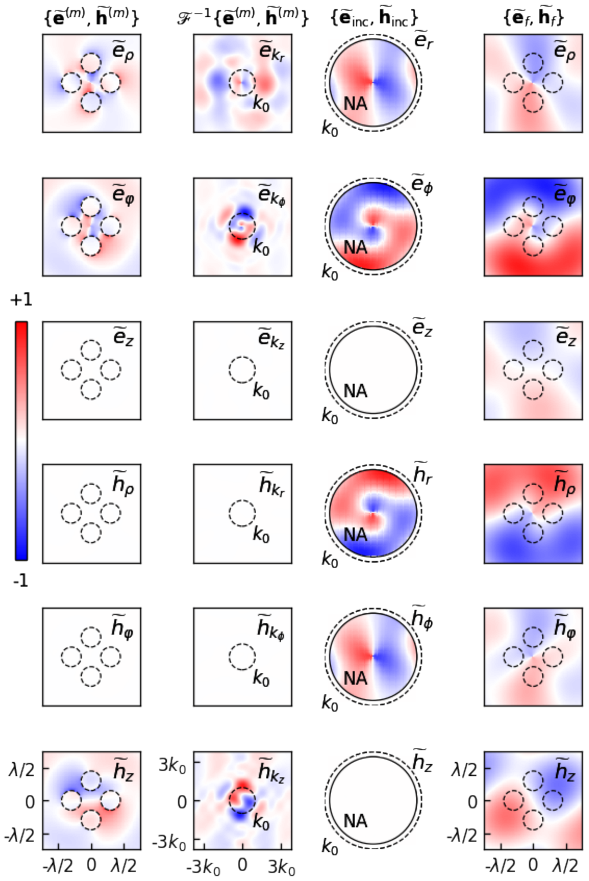


Figure S26. Fields for mode M2 in a nanodisk tetramer.

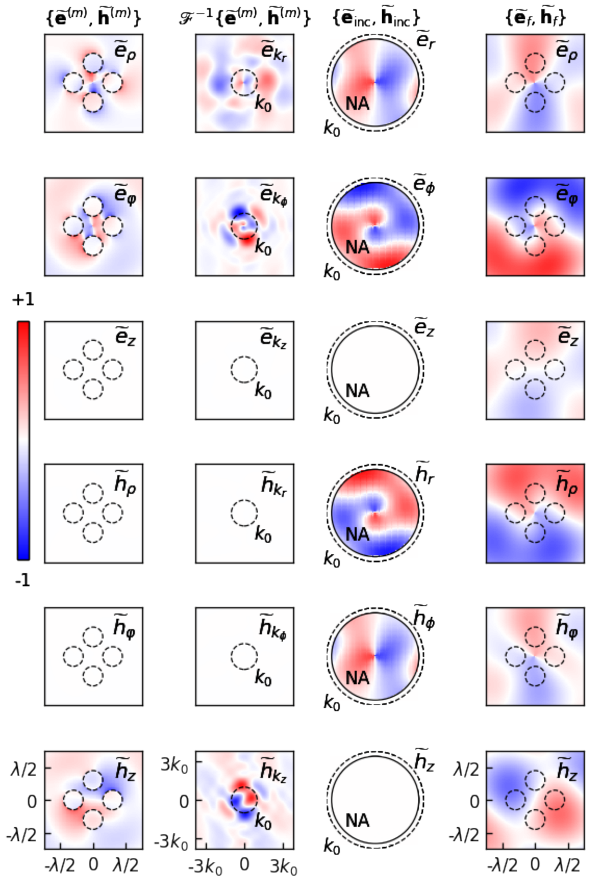


Figure S27. Fields for mode M3 in a nanodisk tetramer.

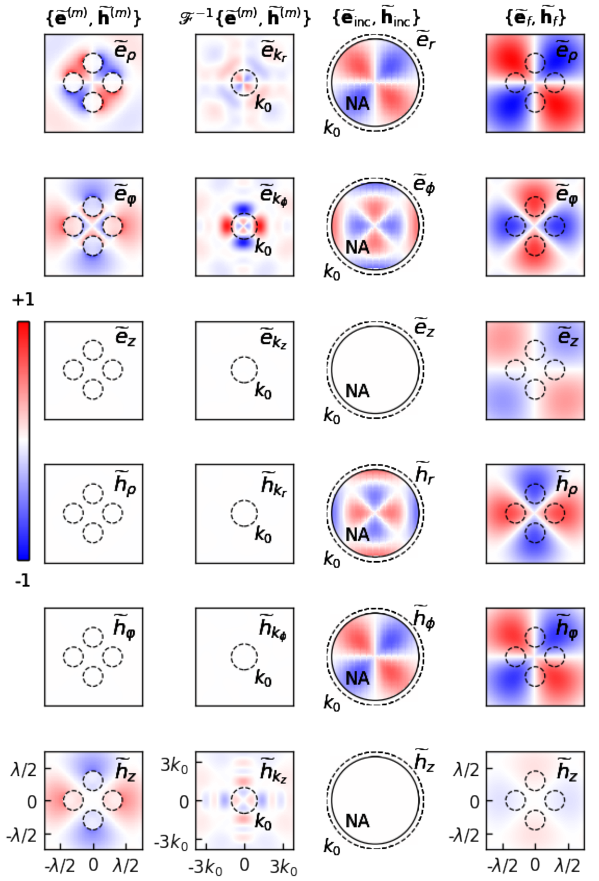


Figure S28. Fields for mode M4 in a nanodisk tetramer.

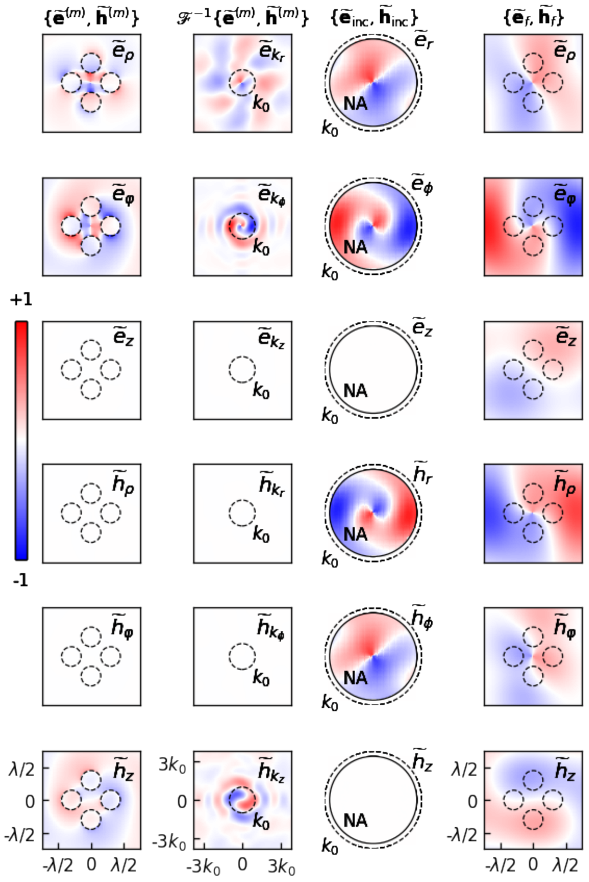


Figure S29. Fields for mode M5 in a nanodisk tetramer.

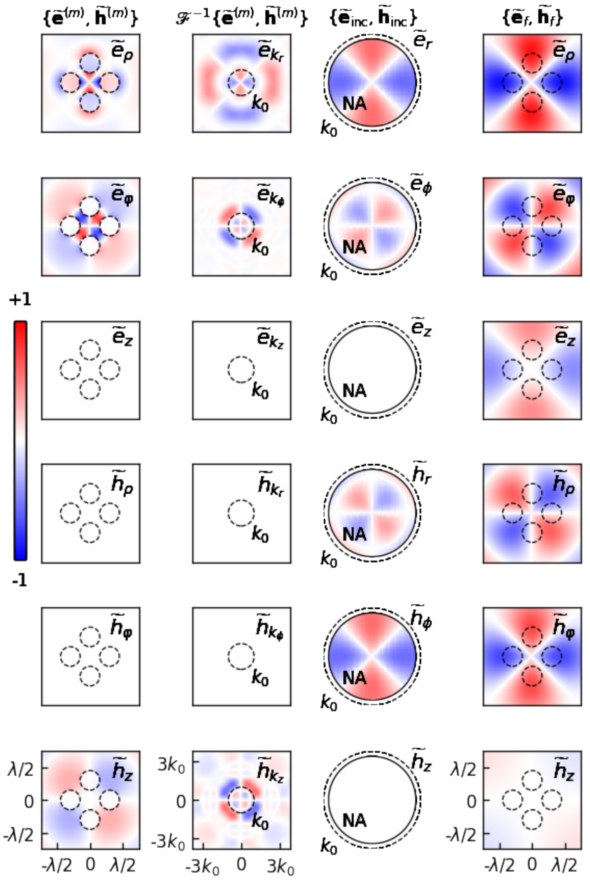


Figure S31. Fields for mode M7 in a nanodisk tetramer.

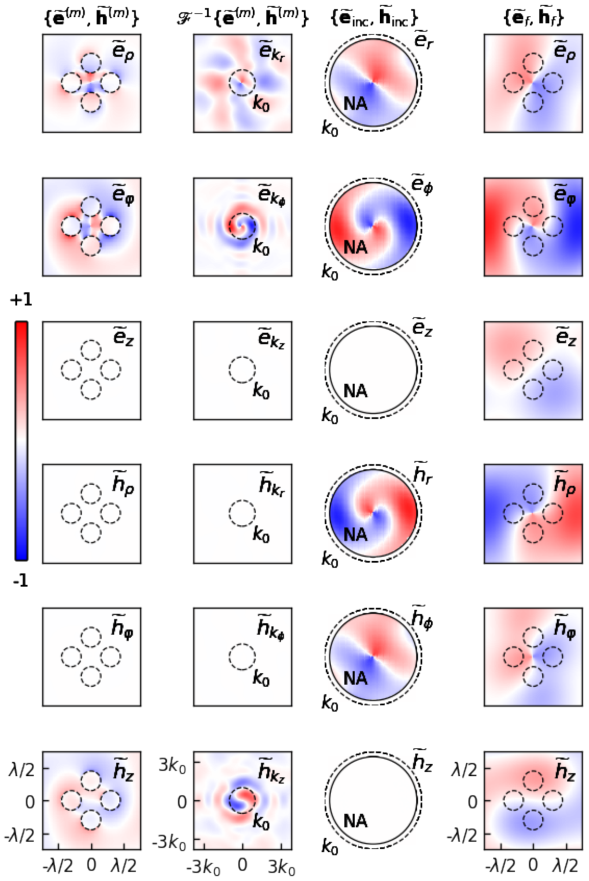


Figure S30. Fields for mode M6 in a nanodisk tetramer.

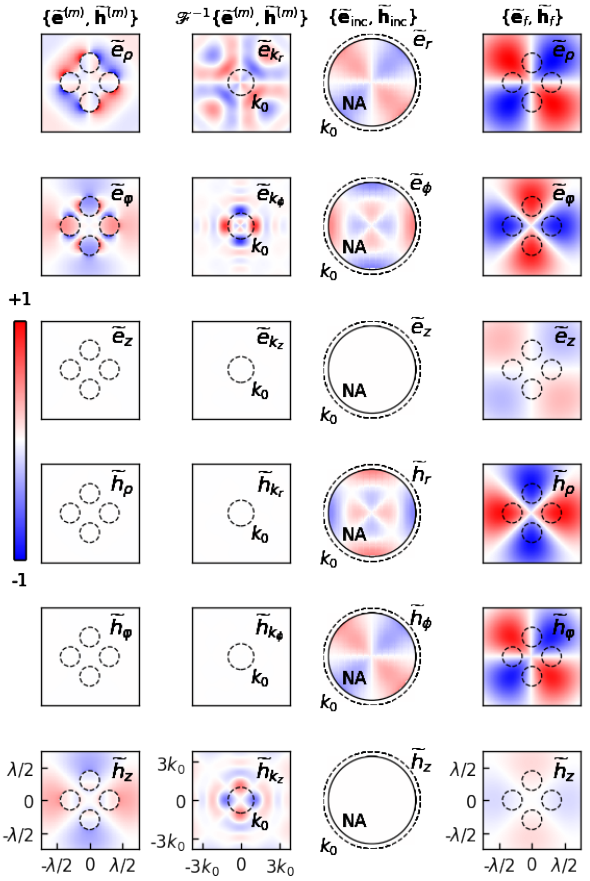


Figure S32. Fields for mode M8 in a nanodisk tetramer.

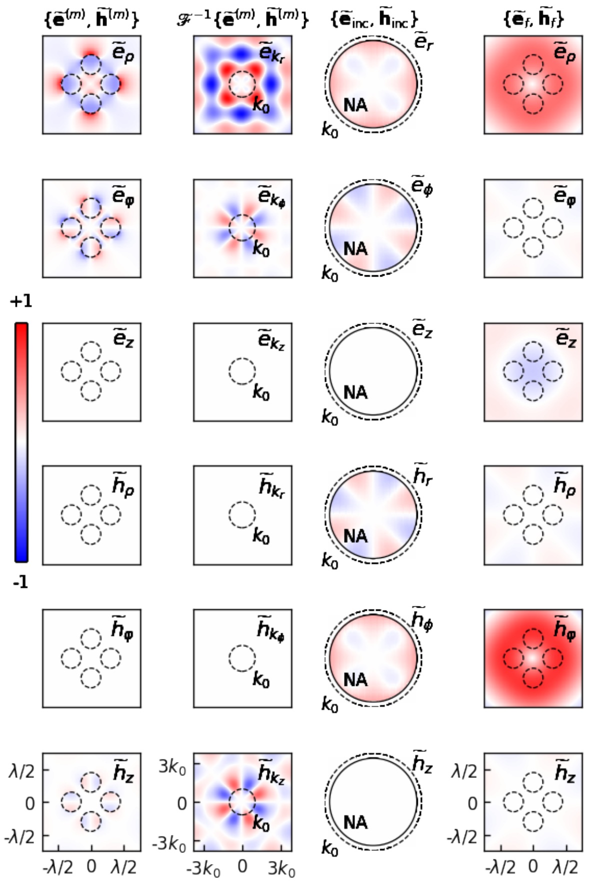


Figure S33. Fields for mode M9 in a nanodisk tetramer.

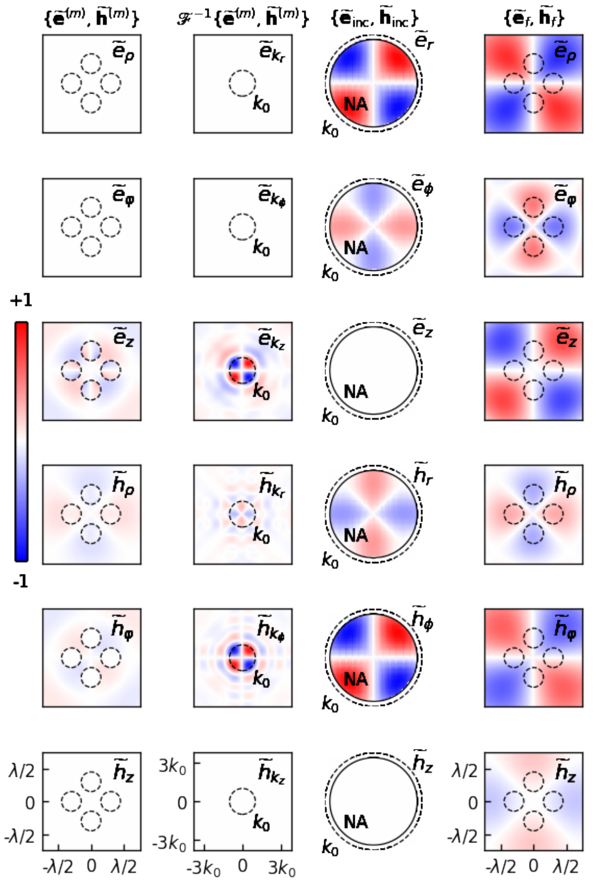


Figure S34. Fields for mode M10 in a nanodisk tetramer.

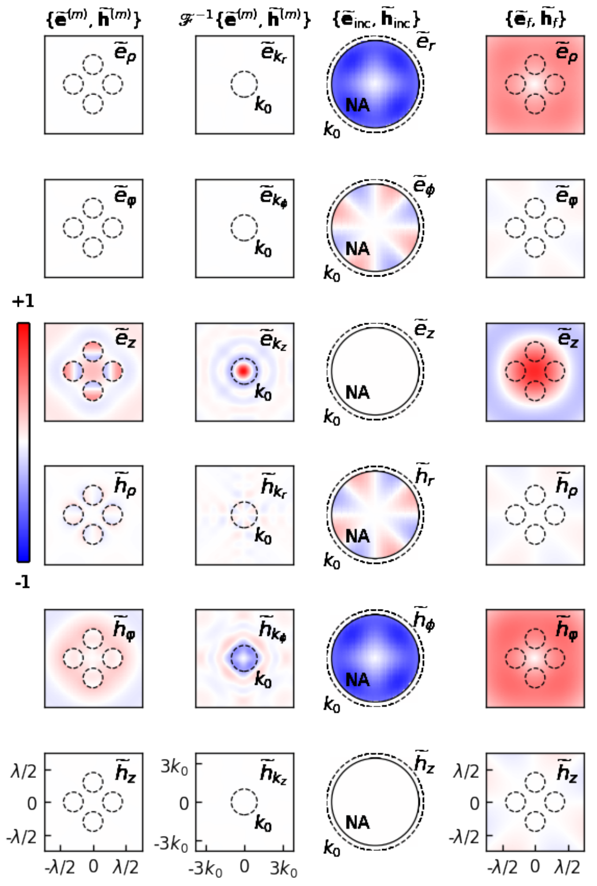


Figure S35. Fields for mode M11 in a nanodisk tetramer.

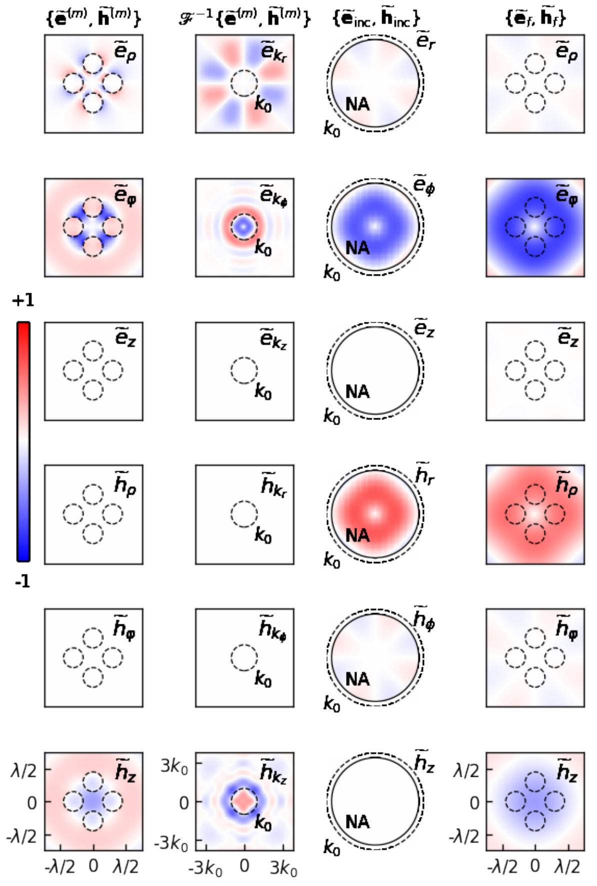


Figure S36. Fields for mode M12 in a nanodisk tetramer.
